# Supplementary material for: Quantifying First-Order Markov Violations in Noisy Reinforcement Learning: A Causal Discovery Approach
Source: arXiv:2503.00206 source file (2025-06-01)
Supplement: Supplementary file 1 [file appendix.tex]

%%%%%%%%%%%%%%%%%%%%%%%%%%%%%%%%%%%%%%%%%%%%%%%%%%%%%%%%%%%%%%%%%%%%%%%%%%%%%%%
\appendix
\section{Implementation \& Reproducibility Details}
\label{app:impl}

\paragraph{Hardware.}  
All experiments ran on a single \textbf{Apple M3 Pro} (12-core CPU, 18 GB unified memory).  
Peak RAM during training never exceeded 4 GB; no GPU or TPU acceleration is required.

\paragraph{Software environment.}

\begin{itemize}
  \item Python 3.11.2
  \item \texttt{stable-baselines3} 2.3.0 (policy optimisation)
  \item \texttt{gymnasium} 0.29.1 (environments)
  \item \texttt{tigramite} 5.2.3 (PCMCI causal discovery)
  \item \texttt{numpy} 1.26.4, \texttt{scipy} 1.12, \texttt{matplotlib} 3.8
\end{itemize}

\noindent
A fresh conda (or venv) install can be reproduced with:
\begin{verbatim}
conda create -n markov python=3.11 -y
conda activate markov
pip install stable-baselines3==2.3.0 gymnasium==0.29.1 \
            tigramite==5.2.3 matplotlib==3.8
\end{verbatim}

\paragraph{Script entry-points.}  
All functionality is exposed through a single orchestrator:

\begin{verbatim}
python markovianess/main.py                 # run the full pipeline
python markovianess/main.py --env CartPole-v1   # one environment only
\end{verbatim}

The orchestrator reads a human-readable \texttt{config.json} file
(specified with \texttt{--config\_path}) that lists
\emph{(i)} environments, \emph{(ii)} training budgets, and  
\emph{(iii)} noise/perturbation grids.
An abridged example is shown below (full version in the supplementary ZIP):
\begin{verbatim}
{
  "environments": [
    {"name":"CartPole-v1", "time_steps":30000,
     "observations":["CartPos","CartVel","PoleAngle","PoleAngVel"],
     "n_envs":1}
  ],
  "noise_strategies": {
    "gaussian": [
      {"mean":0.0, "variance":0.01},
      {"mean":0.0, "variance":0.05}
    ],
    "auto_regressive": {
      "AR(1)":[{"alphas":[0.9], "sigma":0.1}],
      "AR(2)":[{"alphas":[0.9,0.1], "sigma":0.1}]
    }
  }
}
\end{verbatim}

\paragraph{Training hyper-parameters.}  
Across \emph{all} conditions we employ \texttt{PPO} defaults from
\texttt{stable-baselines3}: two 64-unit \textsc{tanh} layers,
Adam with learning rate $3\times10^{-4}$,
discount $\gamma=0.99$, GAE $\lambda=0.95$, clip ratio $0.2$,
entropy coefficient $0$, value-loss coefficient $0.5$, mini-batch 64,
and four optimisation epochs per update.  
\textbf{No hyper-parameter tuning} is performed.

\paragraph{Seed protocol.}  
Every condition (baseline, each noise level, each dimension-drop) is
repeated with five independent seeds following the pattern
$10000\!+\!i$ for $i\in\{0,\dots,4\}$ (identical to the description in
\S\ref{sec:seeds-ci}).  
The orchestrator automatically injects these seeds into
\texttt{gymnasium}, \texttt{stable-baselines3}, NumPy, and Python’s
\texttt{random} module.

\paragraph{Markov-Violation Score (MVS).}  
For each trained policy we collect an additional $1$–$2$ k transitions,
run PCMCI with ParCorr ($\tau_{\max}=5$, $\alpha=0.05$), and compute

\[
  \text{MVS} \;=\;
  \frac{\sum_{k=2}^{5}
        (k-1)\!\!\sum_{i,j}\!\!
        \bigl|\rho_{ij}(k)\bigr|\,
        \bigl[-\ln p_{ij}(k)\bigr]\,
        \mathbf{1}[p_{ij}(k)\le 0.05]}
       {N^{2}\;\sum_{k=2}^{5}(k-1)}.
\]

\noindent
Five independent PCMCI runs are combined with Fisher’s method and
partial-correlation averaging, exactly as in
Algorithm 1 of the main paper.

\paragraph{Running time.}  
End-to-end, one full sweep over the three environments
(\emph{CartPole}, \emph{Pendulum}, \emph{Acrobot})
with all perturbations finishes in \textasciitilde4 h wall-clock on the
above M3 Pro workstation (parallelised over 10\,OS threads).
%%%%%%%%%%%%%%%%%%%%%%%%%%%%%%%%%%%%%%%%%%%%%%%%%%%%%%%%%%%%%%%%%%%%%%%%%%%%%%%
